# Supplementary material for: Making Non-Stochastic Control (Almost) as Easy as Stochastic
Source: arXiv:2006.05910 source file (2020-10-05)
Supplement: Supplementary file 1 [file app_discussion.tex]

%!TEX root = ../so_control_main.tex

	\subsection{Discussion of Results\label{app:comparison_discussion}}
	\input{body/discussion}
	\subsection{Conclusion \label{app:conclusion}}
	\input{body/conclusion}
