# Supplementary material for: Making Non-Stochastic Control (Almost) as Easy as Stochastic
Source: arXiv:2006.05910 source file (2020-10-05)
Supplement: Supplementary file 2 [file app_slow.tex]

%!TEX root = ../main.tex
\section{Slow Rates and Adaptation to Stochastic Settings}
