# Supplementary material for: Making Non-Stochastic Control (Almost) as Easy as Stochastic
Source: arXiv:2006.05910 source file (2020-10-05)
Supplement: Supplementary file 3 [file dfc_background.tex]

%!TEX root = main.tex

To understand the above parametrization, consider the idealized case where $\ypinothat_s = \ypinot_s$, $\upinothat_s = \upinot_s$ are the true inputs/outputs selected by policy $\pi_0$ for all $s \ge 1$, we set $h = \infty$, and $\Ghat = \Gpinot$. Consider the control policy $\pi^M$ which always selects $\utot_t(M\midypinot{t},\maty_{1:t}^M)$ at each round, where $\maty^M_t$ is recursively defined as the iterate produced by such a policy.  \cite{simchowitz2020improper} denomstrate that if $\radcomp,h$ are sufficiently large, there exists an $M \in  \calM$ for which $\Regret_T(\pi^M;\Pistar)$ is small; in otherwords, controls $\utot_t(M\midypinot{t},\maty^M_{1:t})$ well-approximate the optimal controller. 

Up to truncation by the horizon parameter $h$, and estimation errors in $\ypinot,\upinot,\Ghat$, the functions $f_t(M \mid \cdot)$ represents the cost of selecting a fixed policy $\pi^M$ for all $t$. More generally, for a sequence $(M_s)$, $F_t(M_{t:t-h}\mid \cdot)$ represents the cost that would incurred from selecting  $\utot_s(M_s \mid \cdot)$ for all past time $s \le t$.
